# Supplementary material for: Fast and Simple Multiclass Data Segmentation: An Eigendecomposition and Projection-Free Approach
Source: arXiv:2508.09738 ancillary file (2025-12-22)
Supplement: Supplementary file 1 [file Projection_Free_Methods_for_Multiclass_Data_Segmentation_SM.pdf]

# SUPPLEMENTARY MATERIALS: Fast and Simple Multiclass Data Segmentation: An Eigendecomposition and Projection-Free Approach

Chiara Faccio*, Margherita Porcelli†, Francesco Rinaldi†, and Martin Stoll‡

**SM1. Image labeling.** In this section, we provide the explanation of how we generated the ground truth for the image labeling experiments, Subsection SM1.1, as well as the labeling results with their confusion matrices in Subsection SM1.2.

**SM1.1. Generation of the ground truth.** On order to compute the accuracy values for the images, we needed to generate their ground truths, see Figure SM1. In the case of *beach* image, the ground truth was obtained in MATLAB by analyzing the L*a*b color space[1]. For *3 geometric figures*, *4 geometric figures* and *sheets of paper* images, we downloaded the original ground truths from the Visillect's benchmark dataset[2] and we shrank them using the MATLAB command `imresize` with the specified interpolation method "nearest". In this way, each output pixel was assigned the color of the nearest pixel and no other colors were generated, avoiding the gradient color effect.

**SM1.2. Numerical results.** We report the labeling results and their confusion matrices for all the images. Figures SM2-SM7 give a clear qualitative overview of the superiority in the accuracy provided by GSFW (OSFW) with respect to CS and MBO. Figures SM2 and SM3 shows that GFW labels the 3 geometric figures and the background quite well (Fig. SM2(b)), while a piece of the "light blue prism" is labeled as "cube" by CS (Fig. SM2(c)) and MBO completely misses the "light blue prism" (Fig. SM2(d)). In Figures SM4 and SM5, the reconstruction provided by GFW is acceptable (Fig. SM4(b)), while in Fig. SM4(c) the "yellow prism" is labeled as "red pyramid" and in Fig. SM4(d) both the "yellow prism" and the "light blue prism" are not identified. Finally in Figures SM6 and SM7, GFW identifies the colored sheets of papers and the background (Fig. SM6(b)), while the colors are mixed in Fig. SM6(c) (see e.g. the "white paper" and the "pink paper") and in Fig. SM6(d) (see e.g. the "yellow paper").

*Department of Mathematics "Tullio Levi-Civita" University of Padova, Italy (rinaldi@math.unipd.it, chiara.faccio@unipd.it)

†Dipartimento di Ingegneria Industriale (DIEF) Università degli Studi di Firenze, Italy, ISTI–CNR, Italy and member of the INdAM Research Group GNCS (margherita.porcelli@unifi.it)

‡Department of Mathematics, Chemnitz University of Technology, Germany (martin.stoll@math.tu-chemnitz.de)

[1]MATLAB example *Color-Based Segmentation Using the L*a*b* Color Space* https://it.mathworks.com/help/images/color-based-segmentation-using-the-l-a-b-color-space.html

[2]https://github.com/Visillect/colorsegdataset

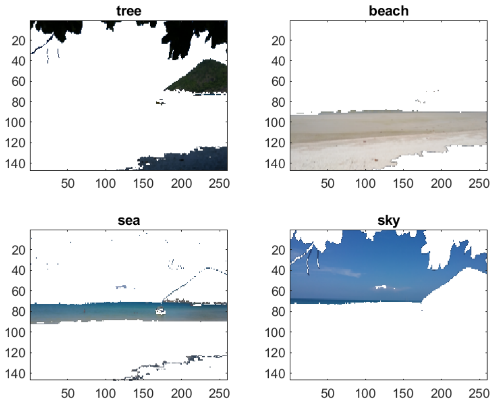


(a) *Beach* image

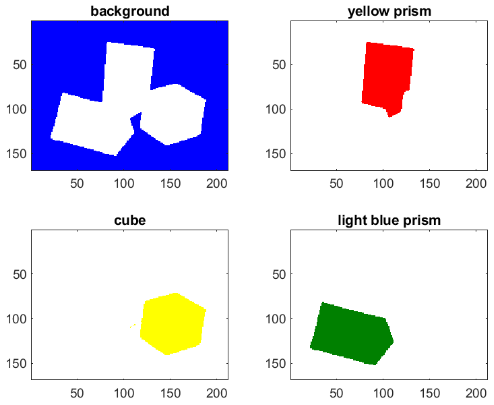


(b) *3 geometric figures* image

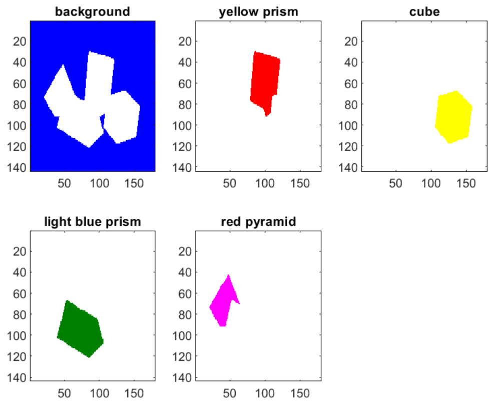


(c) *4 geometric figures* image

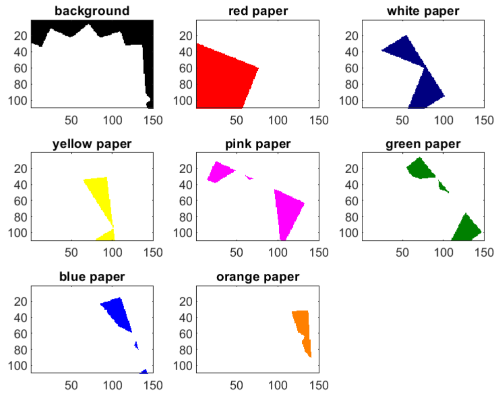


(d) *Sheets of paper* image

Figure SM1: Ground truth for the four images.

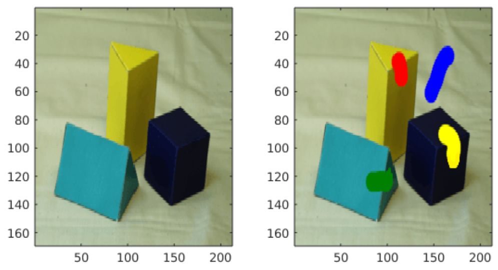

(a) Original (left) and labeled (right) image

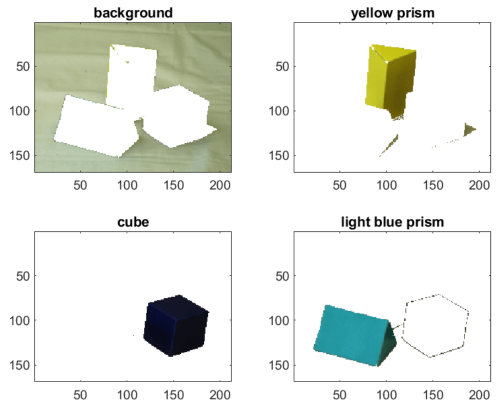


(b) Segmentation with GFW

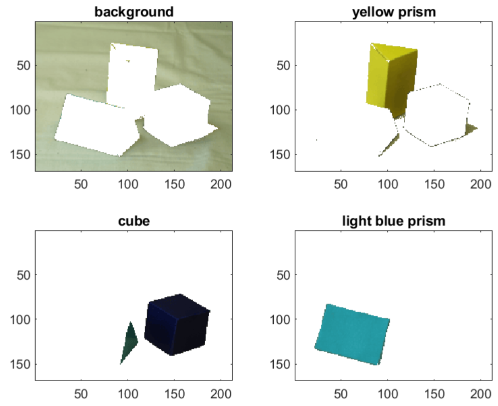


(c) Segmentation with CS

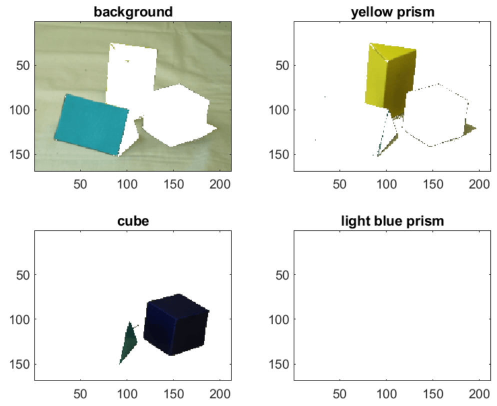


(d) Segmentation with MBO

Figure SM2: *3 geometric figures* image: labeling results with GFW (b), CS (c) and MBO (d).

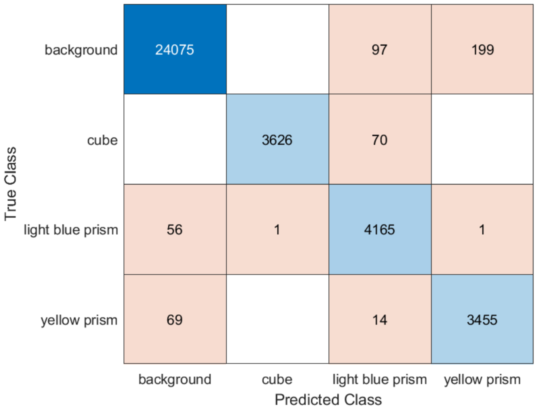


(a) Confusion matrix GFW

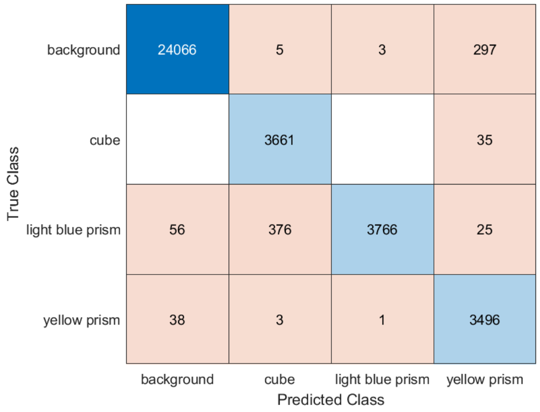


(b) Confusion matrix CS

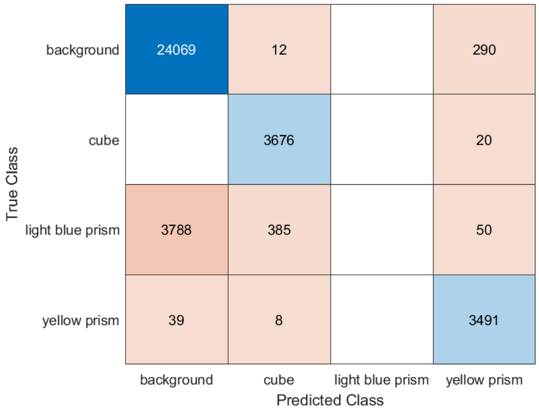


(c) Confusion matrix MBO

Figure SM3: *3 geometric figures* image: confusion matrix results with GFW (a), CS (b) and MBO (c).

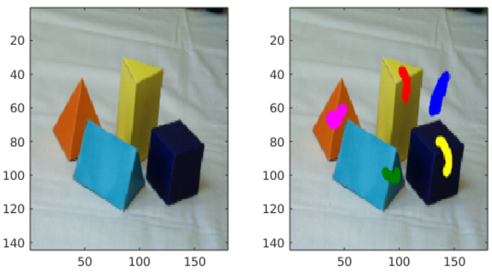

(a) Original (left) and labeled (right) image

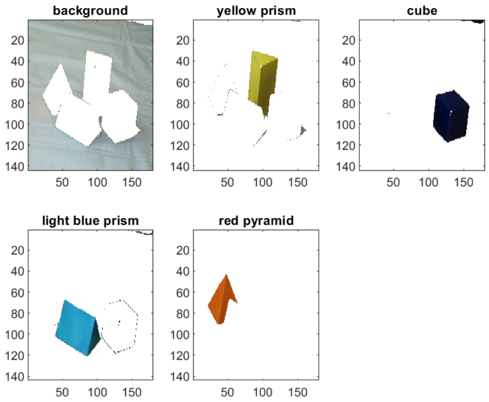


(b) Segmentation with GFW (OSFW)

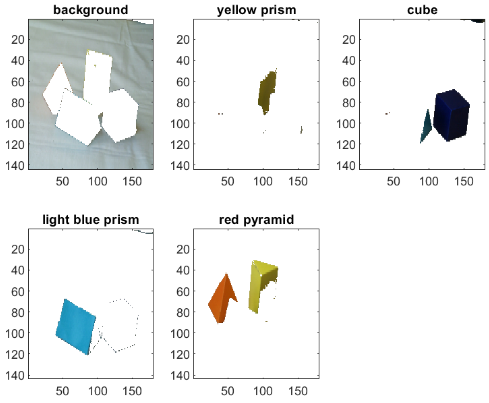


(c) Segmentation with CS

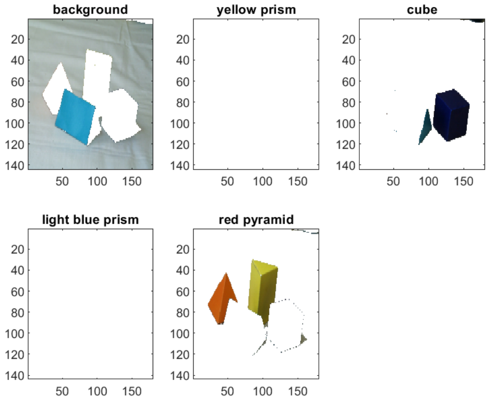


(d) Segmentation with MBO

Figure SM4: *4 geometric figures* image: labeling results with GFW (b), CS (c) and MBO (d).

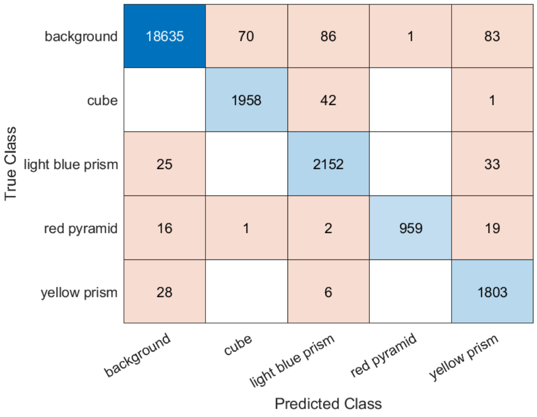


(a) Confusion matrix GFW

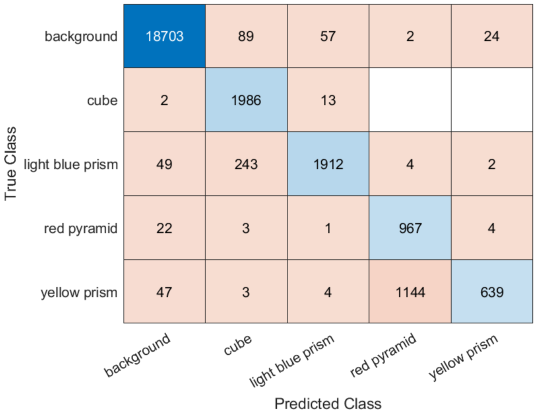


(b) Confusion matrix CS

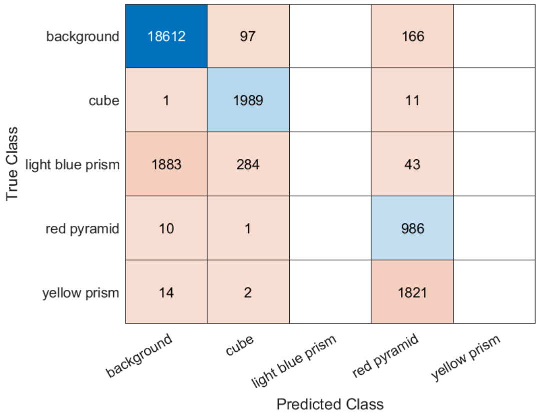


(c) Confusion matrix MBO

Figure SM5: *4 geometric figures* image: confusion matrix results with GFW (a), CS (b) and MBO (c).

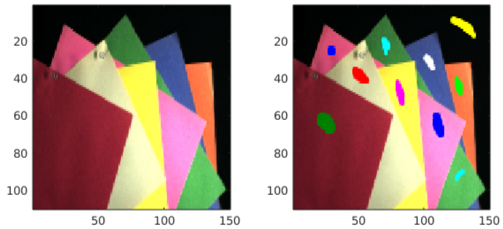

(a) Original (left) and labeled (right) image

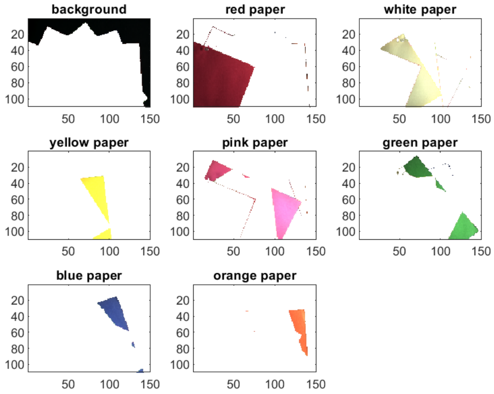


(b) Segmentation with GFW (OSFW)

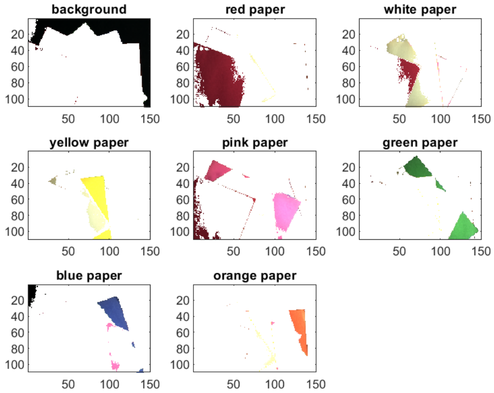


(c) Segmentation with CS

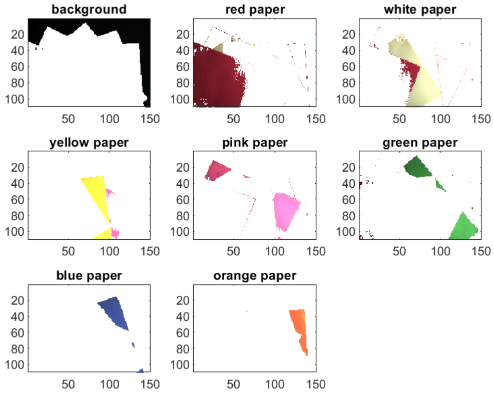


(d) Segmentation with MBO

Figure SM6: *Sheets of paper* image: labeling results with GFW (b), CS (c) and MBO (d).

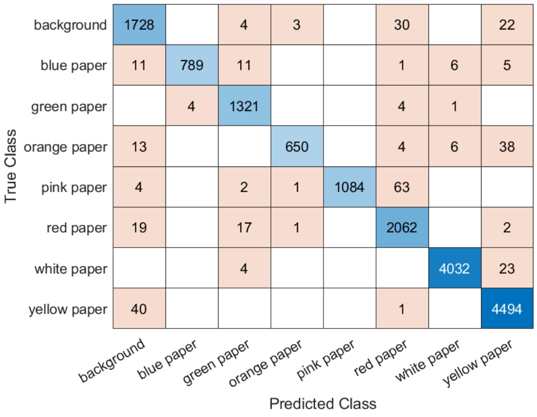


(a) Confusion matrix GFW

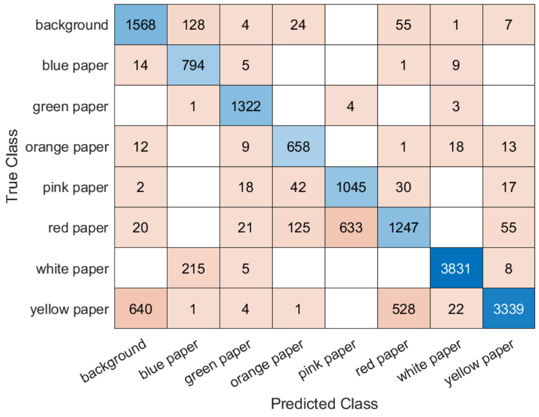


(b) Confusion matrix CS

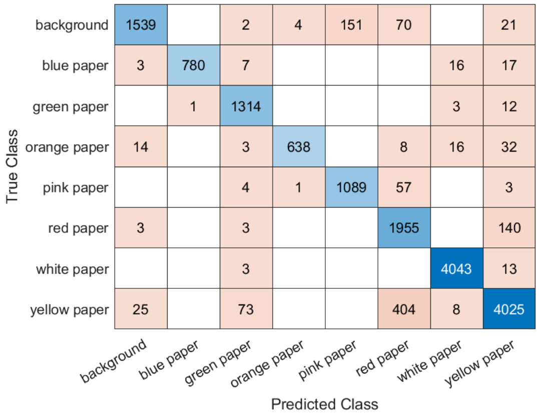


(c) Confusion matrix MBO

Figure SM7: *Sheets of paper* image: confusion matrix results with GFW (a), CS (b) and MBO (c).
